# Supplementary material for: Spectrum Sharing Strategies for UAV-to-UAV Cellular Communications
Source: arXiv:2008.10993 source file (2020-08-18)
Supplement: Supplementary file 1 [file Appendix.tex]

\begin{appendix}

\subsection{Sketch of Proof of Proposition~\ref{proposition:meanUAVtxPower} \newline(see \cite{azari2019uav} for more detailed derivations)} \label{proof:meanUAVtxPower}

The mean UAV transmit power can be written as
\begin{align} \label{eqn:meanPowerProof}
\mathbb{E}[\pu] = \sum_{\nu \in \{\mathrm{L},\mathrm{N}\}}\int_0^\rMuu f_{\Ru}^\nu(\ru) \mathbb{E}\left[\pu^\nu|\Ru = \ru\right]  \mathrm{d}\ru,
\end{align}
where $f_{\Ru}^\nu(\ru) = f_{\Ru}(\ru) \cdot \pruu^\nu(\ru)$ and where the integral in (\ref{eqn:meanPowerProof}) can be written as
\begin{equation} \label{eqn:meanPowerIntegrals}
\begin{aligned}
&\int_0^\rMuu f_{\Ru}^\nu(\ru) \mathbb{E}\left[\pu^\nu|\Ru = \ru\right]  \mathrm{d}\ru \\
&\!=\!\int_0^\mathrm{r_m^\nu} \!f_{\Ru}^\nu(\ru) \mathbb{E}[\rho_\u \zeta_{\u\u}^{\eu}] \, \mathrm{d}\ru \!+\! \int_\mathrm{r_m^\nu}^\rMuu \!f_{\Ru}^\nu(\ru) \mathbb{E}[\pumax]  \mathrm{d}\ru. \! 
\end{aligned}
\end{equation}
The first integral on the right-hand side of (\ref{eqn:meanPowerIntegrals}) is equal to
\begin{equation}
\begin{aligned}
&\int_0^\mathrm{r_m^\nu} \!f_{\Ru}^\nu(\ru) \mathbb{E}[\rho_\u \zeta_{\u\u}^{\eu}] \, \mathrm{d}\ru \\
&=\sum_{i=1}^{j} c_i \int_{\r_i}^\mathrm{r_{i+1}} \ru^{1+\auu^\nu \eu } \cdot e^{-\r_\u^2/(2\sigma_\mathrm{u}^2)}  \mathrm{d}\ru
\end{aligned}
\end{equation}
where 
\begin{align}
c_i &= \frac{\pur\left(\hat{\tau}_{\mathrm{uu}}^\nu/\guu\right)^{\eu}}{\sigma_\u^2[1-\e^{-r_\mathrm{M}^2/(2\sigma_\mathrm{u}^2)}]} \cdot \pruu^\nu(r_i).
\end{align}
With the change of variable $y = \r_\u^2/2\sigma_\mathrm{u}^2$, we can write
\begin{equation}
\begin{aligned}
&c_i^\nu \int_{\r_i}^\mathrm{r_{i+1}} \ru^{1+\auu^\nu \eu } \cdot e^{-\r_\u^2/(2\sigma_\mathrm{u}^2)}  \mathrm{d}\ru \\
%&= C_i^\nu \int_{y_i}^{y_{i+1}} y^{\auu^\nu \eu /2} \cdot e^{-y}  \mathrm{d}y \\
%&= C_i^\nu \left(\int_{0}^{y_{i+1}} y^{\auu^\nu \eu /2} \cdot e^{-y}  \mathrm{d}y - \int_{0}^{y_{i}} y^{\auu^\nu \eu /2} \cdot e^{-y}  \mathrm{d}y \right) \\
& \!= C_i^\nu \Big[ \gamma(1\!+\!\auu^\nu \eu /2,y_{i+1}) \!-\! \gamma(1\!+\!\auu^\nu \eu /2,y_{i}) \Big] \label{eqn:meanPowerFirstIntegral}
\end{aligned}
\end{equation} 
where $y_i = \frac{r_i^2}{2\sigma_u^2}$ and
\begin{align}
C_i^\nu &= \frac{(2\sigma_\u^2)^{{\auu^\nu\eu/2}}\pur\left(\hat{\tau}_{\mathrm{uu}}^\nu/\guu\right)^{\eu}}{1-\e^{-r_\mathrm{M}^2/(2\sigma_\mathrm{u}^2)}} \cdot \pruu^\nu(r_i);~i>0,
\end{align}
thus obtaining
\begin{equation} \label{eqn:meanPowerFirstIntegralResult}
\begin{aligned}
&\int_0^\mathrm{r_m^\nu} f_{\Ru}^\nu(\ru) \mathbb{E}[\rho_\u \zeta_{\u\u}^{\eu}] \, \mathrm{d}\ru \\
& = \sum_{i=1}^{j} [C_i^\nu-C_{i+1}^\nu] \, \gamma(1+\auu^\nu \eu k/2,y_{i+1})
\end{aligned}
\end{equation}
where $C_{j+1}^\nu = 0$. 
Similarly, the second integral on the right-hand side of (\ref{eqn:meanPowerIntegrals}) is equal to
\begin{equation} \label{eqn:meanPowerSecondIntegral}
\int_\mathrm{r_m^\nu}^\rMuu f_{\Ru}^\nu(\ru) \mathbb{E}[\pumax]  \mathrm{d}\ru = \sum_{i=j+1}^{k+1} [B_i^\nu-B_{i-1}^\nu] \, e^{-r_i^2/(2\sigma_\mathrm{u}^2)}
\end{equation}
where $B_j^\nu = 0$, $B_{k+1}^\nu = 0$, and
\begin{align}
B_i^\nu &= \frac{\pumax \, \pruu^\nu(r_i) }{1-\e^{-r_\mathrm{M}^2/(2\sigma_\mathrm{u}^2)}};~i>j.
\end{align}
Proposition~\ref{proposition:meanUAVtxPower} then follows from substituting (\ref{eqn:meanPowerFirstIntegralResult}) and (\ref{eqn:meanPowerSecondIntegral}) into (\ref{eqn:meanPowerIntegrals}) and then into (\ref{eqn:meanPowerProof}).

\subsection{Sketch of Proof of Theorem~\ref{proposition:U2Ucoverage} \newline(see \cite{azari2019uav} for more detailed derivations)} \label{proof:U2Ucoverage}

From Approximation~2, we have $\mathcal{C}_{\mathrm{u}|\Ru}^\N(\ru) = 0$, thus
\begin{equation} \label{eq:U2ULinkCoverage}
\begin{aligned}
\pcovuav &= \sum_{\nu \in \{\mathrm{L},\mathrm{N}\}}\int_0^{\rMuu}  \mathcal{C}_{\mathrm{u}|\Ru}^\nu(\ru)\,f_{\Ru}^\nu(\ru) \,\mathrm{d}\ru \\
&= \int_0^\rMuu f_{\Ru}^\L(\ru) \mathcal{C}_{\mathrm{u}|\Ru}^\L(\ru) \mathrm{d}\ru,
\end{aligned}
\end{equation}
where by using Approximation 1 we can write
%\begin{align} \label{CuRu} \nonumber
%&\mathcal{C}_{\mathrm{u}|\Ru}^\L(\ru) % &\triangleq \mathbb{P}\left[\frac{\pu^\nu \zuu^\nu(\ru)^{-1} \, \suu^\nu}{\mathrm{N_0} + I_\mathrm{u}} > \t \right]\\
%%&\mathcal{C}_{\mathrm{u}|\Ru}^\nu(\ru) 
%%&= \mathbb{P}\left[\frac{\pu^\nu \zuu^\nu(\ru)^{-1} \, \suu^\nu}{\mathrm{N_0} + I_\mathrm{u}} > \t \right] \\ \nonumber
%= \mathbb{E}_{I_\mathrm{u}} \left\{\mathbb{P}\left[\suu^\L > \frac{\t}{\pu^\L \zuu^\L(\ru)^{-1}}(\mathrm{N_0} + I_\mathrm{u}) \right] \right\} \\ \nonumber
%&= 1 -  \mathbb{E}_{I_\mathrm{u}} \left\{\mathbb{P}\left[\suu^\L < \frac{\t}{\pu^\L \zuu^\L(\ru)^{-1}}(\mathrm{N_0} + I_\mathrm{u}) \right] \right\} \\ \nonumber
%&\approx \mathbb{E}_{\iu} \left\{\sum_{i=1}^{\mathrm{m_{uu}^\L}} \binom{\mathrm{m_{uu}^\L}}{i}(-1)^{i+1} e^{-z_{\u,i}^\L (\mathrm{N_0} + I_\mathrm{u})} \right\} \\ \nonumber
%&= \sum_{i=1}^{\mathrm{m_{uu}^\L}} \binom{\mathrm{m_{uu}^\L}}{i}(-1)^{i+1} e^{-z_{\u,i}^\L \mathrm{N_0}} \cdot \mathbb{E}_{\iu}\left\{e^{-z_{\u,i}^\L I_\mathrm{u}} \right\} \\ 
%&= \sum_{i=1}^{\mathrm{m_{uu}^\L}} \binom{\mathrm{m_{uu}^\L}}{i}(-1)^{i+1} e^{-z_{\u,i}^\L \mathrm{N_0}} \cdot \lapiu^\L(z_{\u,i}^\L).
%\end{align}
\begin{equation} \label{CuRu}
\begin{aligned}
\mathcal{C}_{\mathrm{u}|\Ru}^\L(\ru) &\!=\! \mathbb{E}_{I_\mathrm{u}} \!\left\{\mathbb{P}\left[\suu^\L > \frac{\t}{\pu^\L \zuu^\L(\ru)^{-1}}(\mathrm{N_0} \!+\! I_\mathrm{u}) \right] \right\} \\
&\!\!= \sum_{i=1}^{\mathrm{m_{uu}^\L}} \binom{\mathrm{m_{uu}^\L}}{i}(-1)^{i+1} e^{-z_{\u,i}^\L \mathrm{N_0}} \cdot \lapiu^\L(z_{\u,i}^\L).
\end{aligned}
\end{equation}
Under Approximation~2, we can neglect the interference generated by NLoS links and obtain
%, i.e., $I_\u = I_{\u\u} + I_{\g\u}$. Therefore,
\begin{equation} \label{eqn:LaplacianProofTheoremOne}
\lapiu^\L(z_{\u,i}^\L) = e^{ -2 \pi (\hat{\lambda}_\u \mathcal{I}_\mathrm{uu}^\L + \lamb \mathcal{I}_\mathrm{gu}^\L)}.
\end{equation}

Theorem~\ref{proposition:U2Ucoverage} then follows by deriving $\mathcal{I}_\mathrm{uu}^\L$ and $\mathcal{I}_\mathrm{gu}^\L$ (with an approach similar to the one in \cite{AzaGerGar19}), by replacing $\pu$ with its mean (from Proposition~\ref{proposition:meanUAVtxPower}), and by substituting $\mathcal{I}_\mathrm{uu}^\L$ and $\mathcal{I}_\mathrm{gu}^\L$ into (\ref{eqn:LaplacianProofTheoremOne}), (\ref{CuRu}), and (\ref{eq:U2ULinkCoverage}).

\end{appendix}
